# Supplementary material for: A Syntactic Approach to Studying Strongly Equivalent Logic Programs
Source: arXiv:2011.04454 source file (2021-12-06)
Supplement: Supplementary file 1 [file appendix.tex]

%!TEX root = lpmln_qsr_se.tex

\newpage
\section*{Appendix: Proofs of Main Results}

\setcounter{table}{0} 
\subsection{A Proof of Table \ref{tab:single-del-sat}}
\input{proofs/single-deletion-sat-table1.tex} 

\subsection{A Proof of Table \ref{tab:single-del-sat-2}}
\input{proofs/single-deletion-sat-table2.tex} 

\subsection*{A Proof of Lemma \ref{lem:single-deletion-non-se}}
\input{proofs/lem-single-deletion-non-se.tex}

\newpage
\input{proofs/thm-no-more-iset-condition.tex}

% \subsection*{A Proof of Lemma \ref{lem:single-deletion}}
% \input{proofs/lem-single-deletion.tex}

% \subsection*{A Proof of Lemma \ref{lem:single-addition}}
% \input{proofs/lem-single-addition.tex}

% \newpage
% \input{proofs/single-ops-sat-table.tex}
